# Supplementary material for: i-Algebra: Towards Interactive Interpretability of Deep Neural Networks
Source: arXiv:2101.09301 source file (2021-01-22)
Supplement: Supplementary file 1 [file appendix.tex]

\section*{Appendix}

% \subsubsection{\bf Definition of Shapley Value\\}
% \label{apdx:shapley}

% A line of work has developed interpretation methods based on Shapley value \cite{shap,Ancona:2019:icml,Chen:2019a:iclr,kononenko2010efficient}.
% Formally, the definition of Shapley value can be given as: let $N$ denotes the set of all input features and $S$ means a subset of features as $S \subseteq N$. A Shapley value based interpreter assigns an important value to each feature as $\phi_i$ that represents the effect of model $f$'s prediction. 
% Specifically, the importance score of each feature $\phi_i$ is computed by the \emph{average marginal contribution} of feature $i$ to all possible coalitions of $S$ that can be formed without it, which can be formed as:

% \begin{equation}
%     \phi_{i}=\sum_{S \subseteq N \backslash\{i\}} \frac{|S| !(|N|-|S|-1) !}{|P| !}[f(S \cup\{i\})-f(S)]
% \end{equation}

% Furthermore, we can view Shapley value from another angle. To compute the importance score $\phi_i$, 
% consider a given coalitions size as $k$, where $0 \leq k \leq N-1$, the expected target output difference with and without feature $i$ is $\mathbb{E}_{S} [ f(x_S \cup \{i\} ) -f(x_S) ]$, so the Shapley value can be reformulated as:

% \begin{equation}
%     \phi_{i} = \frac{1}{N} \sum_{k=0}^{N-1} \mathbb{E}_{S}\left[f\left(x_{S \cup\{i\}}\right)-f\left(x_{S}\right)\right]
% \end{equation}

\subsection*{A. Instantiation of \system for other interpretation methods}
\label{apdx:ialgbra-interpreter}

Besides its instantiation within the Shapley value framework, next we discuss the implementation of \system using other interpretation methods. Without loss of generality, we consider two representative interpretation methods, IntegratedGrad\mcite{Sundararajan:2017:icml} and SmoothGrad\mcite{Smilkov:iclr:2017}.

\vspace{2pt}
\subsubsection*{B1. IntegratedGrad -- }
% Besides its instantiation within Shapley value framework provided, next we also exemplify \system with another representative interpreter named Integrated Gradients proposed in \cite{Sundararajan:2017:icml}, this can further be generated to other interpreters with baseline image setting (e.g., Mask \cite{fong:mask}).

\textbf{Identity.} Within the IntegratedGrad framework, the \emph{identity} operator $\phi(x; \bar{x}, f)$ can be defined as the basic IntegratedGrads interpreter to generate the attribution map as:
\begin{equation}
    [\phi(x)]_i = \left(x_{i}-\bar{x}_{i}\right) \times \int_{\alpha=0}^{1} \frac{\partial f\left(\bar{x}+\alpha \times\left(x-\bar{x}\right)\right)}{\partial x_{i}} d \alpha
\end{equation}

Moreover, in practice, the integral of IntegratedGrads can be efficiently approximated via a summation of $K$ steps defined as:
\begin{equation}
    [\phi(x)]_i = \left(x_{i}-\bar{x}_{i}\right) \times \frac{1}{K} \sum_{k=1}^{K} \frac{\left.\partial f\left(\bar{x}+\frac{K}{m} \times\left(x-\bar{x}\right)\right)\right)}{\partial x_{i}}
\end{equation}

\textbf{Projection.} Within the IntegratedGrad framework, given the window $w$ (on $x$) selected by the user, we also marginalize the part of $x$ outside the window $w$ with the baseline input $\bar{x}$, and thus the \emph{projection} operator $\Phi_w(x)$ generates the local importance of $x$'s features as:
\begin{align}
    \label{eq:prj}
    [\Pi_w(x)]_i =  \left\{
    \begin{array}{cl}
        \left(x_{i}-\bar{x}_{i}\right) \times \frac{1}{K} \sum_{k=1}^{K} \frac{\left.\partial f\left(\bar{x}+\frac{K}{m} \times\left(x-\bar{x}\right)\right)\right)}{\partial x_{i}} & i \in w \\
    0 & i \not\in w
    \end{array}
    \right.
\end{align}

\textbf{Selection.} Within the IntegratedGrad framework, given the input $x$, the $n$ layer DNN model $f_{[1:n]}$ and the layer index $l$ selected by the user, the \emph{join} operator $\sigma_l(x)$ generates attribution map at the l-th layer as below: 

\begin{align}
    \label{op:selection}
        [\sigma_l(x)]_i = [\phi(x; \bar{x}, f_l)]_i = \left(x_{i}-\bar{x}_{i}\right) \times \frac{1}{K} \sum_{k=1}^{K} \frac{\left.\partial f_l \left(\bar{x}+\frac{K}{m} \times\left(x-\bar{x}\right)\right)\right)}{\partial x_{i}}
\end{align}

\textbf{Join ($x \bowtie x'$). }Within the IntegratedGrads framework, the \emph{join} operator computes the most informative features shared by $x$ and $x'$ in similar manner to the Shapley value framework in Eq \ref{op:join} as below:

\begin{align}
[x \bowtie x']_i = \epsilon \cdot [\phi(x; \bar{x}, f)]_i + (1-\epsilon) \cdot [\phi(x'; \bar{x}, f)]_i
\end{align}

\textbf{Anti-Join ($x \ajoin x'$). }Within the IntegratedGrads framework, \emph{anti-join} operator  $x \ajoin x'$ of two inputs $x$ and $x'$ also highlights the most discriminative features similar to the Shapley value framework as defined in Eq \ref{op:ajoin}.

\begin{align}
[x \ajoin x']_i = ([\phi(x; x', f)]_i, [\phi(x'; x, f)]_i)
\end{align}

Additionally, another possible implementation of \emph{anti-join} operator within the IntegratedGrads framework can also be defined as:

\begin{align}
    [x \ajoin x']_i = ([\phi(x; \bar{x}, f)]_i, [\phi(x'; \bar{x}, f)]_i)
\end{align}

\vspace{2pt}
\textbf{B2. SmoothGrad}

In contrast, we further discuss how to extend \system to interpreters without baseline image setting such as GradSaliency \cite{gradsaliency} and SmoothGrad \cite{Smilkov:iclr:2017}, etc. We exemplify \system within the SmoothGrad framework below.

\textbf{Identity ($\phi$).} Within the SmoothGrad framework, the \emph{identity} operator $\phi(x;f)$ can be defined as the basic SmoothGrad interpreter to generate teh attribution map as:

\begin{equation}
    [\phi(x)]_i = \frac{1}{n} \sum_{1}^{n} f\left(x+\mathcal{N}\left(0, \sigma^{2}\right)\right)
\end{equation}

where n defines the number of samples, and $N(0, \sigma^2)$ represents Gaussian noise with standard deviation $\sigma$. These hyperparameters can be assigned by users, otherwise, they will adopt default sets within \system.

\textbf{Projection ($\Pi$).} Within the SmoothGrad framework, user also provides window parameters $w$ on $x$, and \emph{projection} operator replaces the features outside the window $w$ with a \system inherent baseline setting $x_0$ (e.g., all-zero vector), then feed the revised input into model $f$. Thus it generates the attribution map as:

\begin{align}
    \label{eq:prj}
    [\Pi_w(x)]_i =  \left\{
    \begin{array}{cl}
        \frac{1}{n} \sum_{1}^{n} f\left(x+\mathcal{N}\left(0, \sigma^{2}\right)\right) & i \in w \\
        f(x_0) & i \not\in w
    \end{array}
    \right.
\end{align}

\textbf{Selection ($\sigma$). }Within the SmoothGrad framework, given the input $x$, the $n$ layer DNN model $f_{[1:n]}$ and the layer index $l$ selected by the user, the \emph{join} operator $\sigma_l(x)$ generates attribution map at the l-th layer as below: 

\begin{align}
    \label{op:selection}
        [\sigma_l(x)]_i = [\phi(x; \bar{x}, f_l)]_i = \frac{1}{n} \sum_{1}^{n} f_l \left(x+\mathcal{N}\left(0, \sigma^{2}\right)\right)
\end{align}

\textbf{Join ($x \bowtie x'$). }Within the SmoothGrad framework, the \emph{join} operator $x \bowtie x'$ computes the most informative features shared by $x$ and $x'$ in the manner that defined as below:

\begin{align}
    [x \bowtie x']_i = \epsilon \cdot [\phi(x; x', f)]_i + (1-\epsilon) \cdot [\phi(x'; x, f)]_i
\end{align}

\textbf{Anti-Join ($x \ajoin x'$). }Within the SmoothGrad framework, the \emph{anti-join} operator $x \ajoin x'$ computes the most discriminative features of two inputs $x$ and $x'$ using the definition as:

\begin{align}
    [x \ajoin x']_i = ([\phi(x; f)]_i, [\phi(x'; x, f)]_i)
\end{align}

Overall, the \system instantiations of IntegratedGrads and SmoothGrad above aim to shed light on how \system can be flexibly applied to a wide range of existing interpreters covering both with and without baseline interpretation methods \cite{shap,Ancona:2019:icml,Chen:2019a:iclr,kononenko2010efficient,Sundararajan:2017:icml,Smilkov:iclr:2017,fong:mask,gradsaliency}.

% \subsubsection{\bf Survey Results of User Needs on IDLSes\\}
% \label{apdx:survey}

% Here we show the survey results of user needs on IDLSes in Figure \ref{fig:user_survey}.

% \begin{figure}[!ht]
% 	\centering
% 	\epsfig{file = 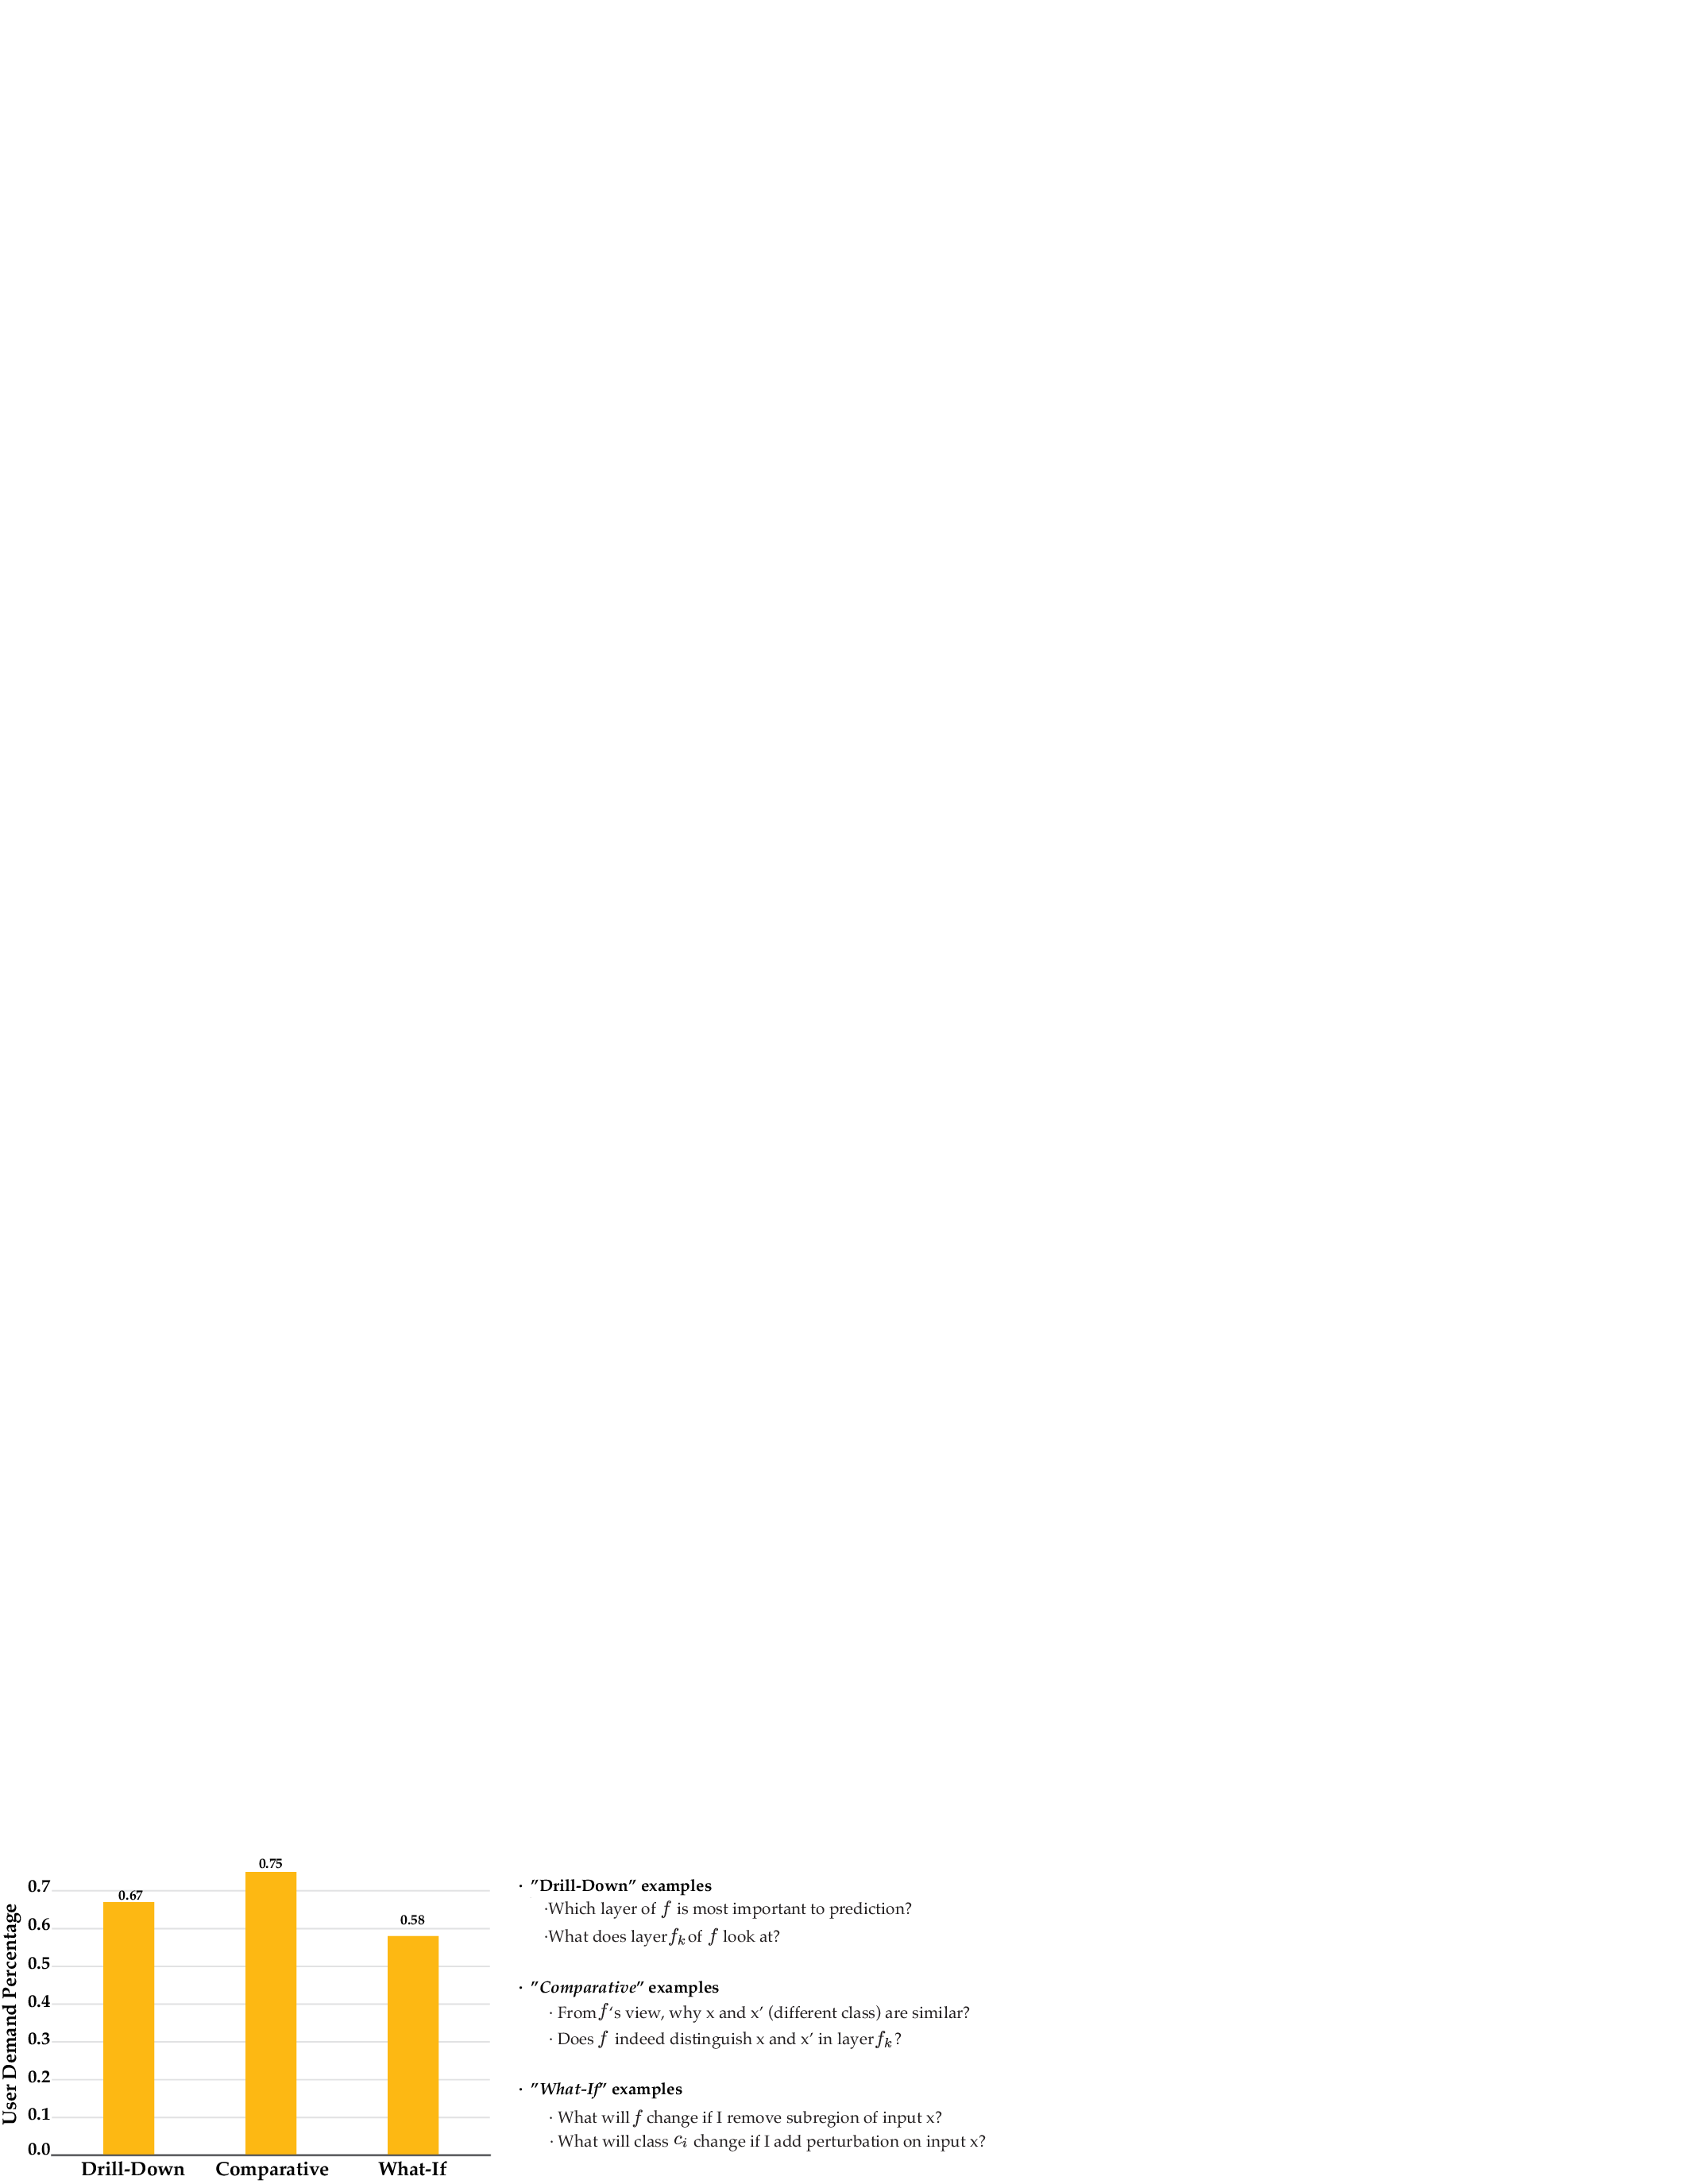, width=85mm}
% 	\caption{Survey statistics of user needs for DNN interpretation. \label{fig:user_survey}}
% \end{figure}

\subsubsection{\bf Declarative Queries in User Studies\\}
\label{apdx:query}

The hints of declarative query for first-time users in all user studies are summarized as below.

\textbf{D1. Use Case A: Resolving Model Inconsistency}

Use case A applies the \emph{Anti-Join} operator to on $x$'s with respect to two different models.

\begin{minted}[mathescape,
    escapeinside=||,
    fontsize=\small,
    ]{sql}
select l from f(x) where w
\end{minted}

\textbf{D2. Use Case B: Detecting Adversarial Inputs}

Use case B applies the \emph{Selection} and \emph{Projection} operators to generates interpretation at different inference stages and various input granularities.

\begin{minted}[mathescape,
    escapeinside=||,
    fontsize=\small,
    ]{sql}
select * from f(x) left join (select * from f|'|(x))
\end{minted}

\textbf{D3. Use Case C: Cleansing Poisoning Data}

Use case C applies the \emph{Selection} operator to examine $x$'s interpretation at the $l-$ layer of $f$.

\begin{minted}[mathescape,
    escapeinside=||,
    fontsize=\small,
    ]{sql}
select l from f(x)
\end{minted}
which examines $x$'s interpretation at the $l$-th layer of $f$ (where $l$ is set to be the penultimate layer).

\subsection*{B. Composition of Atomic Operators}

Table\mref{tab:compositions} summarizes the compositions of atomic operators in \system and their important properties.

\begin{table*}[!ht]{\footnotesize
    \setlength\tabcolsep{0.5pt}
    \setlength\extrarowheight{2.5pt}
            \centering
            \begin{tabular}{c|c|c|c|c}
         & {Projection} ($\Pi$)  & {Selection} ($\sigma$) & {Join} ($\bowtie$) & {Anti-Join} ($\ajoin$) \\
        \hline
        \hline

        %\multirow{3}{*}{Projection}      & \emph{Projection} $\cdot$ \emph{Projection}        & \emph{Projection} $\cdot$ \emph{Selection}         & \emph{Projection} $\cdot$ \emph{Join}          & \emph{Projection} $\cdot$ \emph{(Anti-)Join}     \\

 Projection    & $\Circle$ \textbf{Commutative:}                &  $\Circle$ \textbf{Commutative:}    &   $\LEFTcircle$ \textbf{Conditional:}   &   $\LEFTcircle$ \textbf{Conditional:}  \\
 ($\Pi$)     &  $\Pi_{w}\Pi_{w'}(x) = \Pi_{w'}\Pi_{w}(x) = \Pi_{w \cap w'}(x)$     &  $\Pi_{w}\sigma_l(x) = \sigma_l \Pi_w(x)$  &   $w = w'$ in $ \Pi_w(x) \bowtie \Pi_{w'}(x')$    &  $w = w'$ in $ \Pi_w(x) \ajoin \Pi_{w'}(x')$     \\
         \hline

        %\multirow{2}{*}{Selection}      & \emph{Selection} $\cdot$ \emph{Projection}          & \emph{Selection} $\cdot$ \emph{Selection}          & \emph{Selection} $\cdot$ \emph{Join}          & \emph{Selection} $\cdot$ \emph{(Anti-)Join}     \\
     Selection    & $\Circle$  \textbf{Commutative:}      &  $\LEFTcircle$ \textbf{Conditional:}  &  \multirow{2}{*}{$\Circle$  }   &    \multirow{2}{*}{$\Circle$ }  \\
        ($\sigma$)   &   $\Pi_{w}\sigma_l(x) = \sigma_l \Pi_w(x)$  &  $l \leq l'$ in $\sigma_{l}\sigma_{l'}(x)$  &     &      \\
         \hline

        %\multirow{2}{*}{Join}  & \emph{Join} $\cdot$ \emph{Projection}    & \emph{Join} $\cdot$ \emph{Selection}   & \emph{Join} $\cdot$ \emph{Join}    & \emph{Join} $\cdot$ \emph{(Anti-)Join}     \\
       Join  & $\Circle$  \textbf{Distributive:}   & $\Circle$  \textbf{Distributive:}   &  $\Circle$  \textbf{Associative:}       &    \multirow{2}{*}{$\CIRCLE$}    \\
       ($\bowtie$)   & $\Pi_w  (x \bowtie x') = \Pi_w(x) \bowtie \Pi_{w}(x')$   &  $\sigma_l  (x \bowtie x') = \sigma_l(x) \bowtie \sigma_l(x')$  &  $(x_1 \bowtie x_2) \bowtie x_3 = x_1 \bowtie (x_2 \bowtie x_3)$    &      \\
         \hline

        %\multirow{2}{*}{Anti-Join}  & \emph{(Anti-)Join} $\cdot$ \emph{Projection}    & \emph{(Anti-)Join} $\cdot$ \emph{Selection}   & \emph{(Anti-)Join} $\cdot$ \emph{Join}    & \emph{(Anti-)Join} $\cdot$ \emph{(Anti-)Join}     \\
        Anti-Join  &  $\Circle$ \textbf{Distributive:}        & $\Circle$ \textbf{Distributive:}  &  \multirow{2}{*}{$\CIRCLE$}     &  $\Circle$ \textbf{Associative:}       \\
        ($\ajoin$)  &  $\Pi_w  (x \ajoin x') = \Pi_w(x) \ajoin \Pi_{w}(x')$   & $\sigma_l  (x \ajoin x') = \sigma_l(x) \ajoin \sigma_l(x')$    &     & $(x_1\ajoin x_2) \ajoin x_3  =  x_1 \ajoin (x_2 \ajoin x_3)$ \\
        \hline

            \end{tabular}
            \caption{Important properties of the compositions of atomic operators in \system ($\CIRCLE$ -- undefined, $\LEFTcircle$ -- conditional, $\Circle$ -- unconditional).
            \label{tab:compositions}}}
\end{table*}

% \subsubsection{\bf Benign and adversarial inputs with interpretation by \system\\}
% \label{apdx:adversarial}

% User case B compares a set of benign and adversarial inputs, their baseline interpretation, and their interpretation under \system shown in Figure \ref{fig:adv-all}.

% \begin{figure*}[ht]
%  	\centering
%  	\epsfig{file = , width=150mm}
%      \caption{Sample benign and adversarial inputs and their interpretation: (a) benign inputs and baseline interpretation; (b) adversarial inputs and baseline interpretation; (c) benign inputs and \system interpretation; (d) adversarial inputs and \system interpretation. 
%      \label{fig:adv-all}}
% \end{figure*}

% \subsubsection{\bf Distribution of URT in Case C\\}
% \label{apdx:casec}

% Figure \ref{fig:usecasec} shows the distribution of URT for use case C.

% \begin{figure*}[!ht]
% 	\epsfig{file = 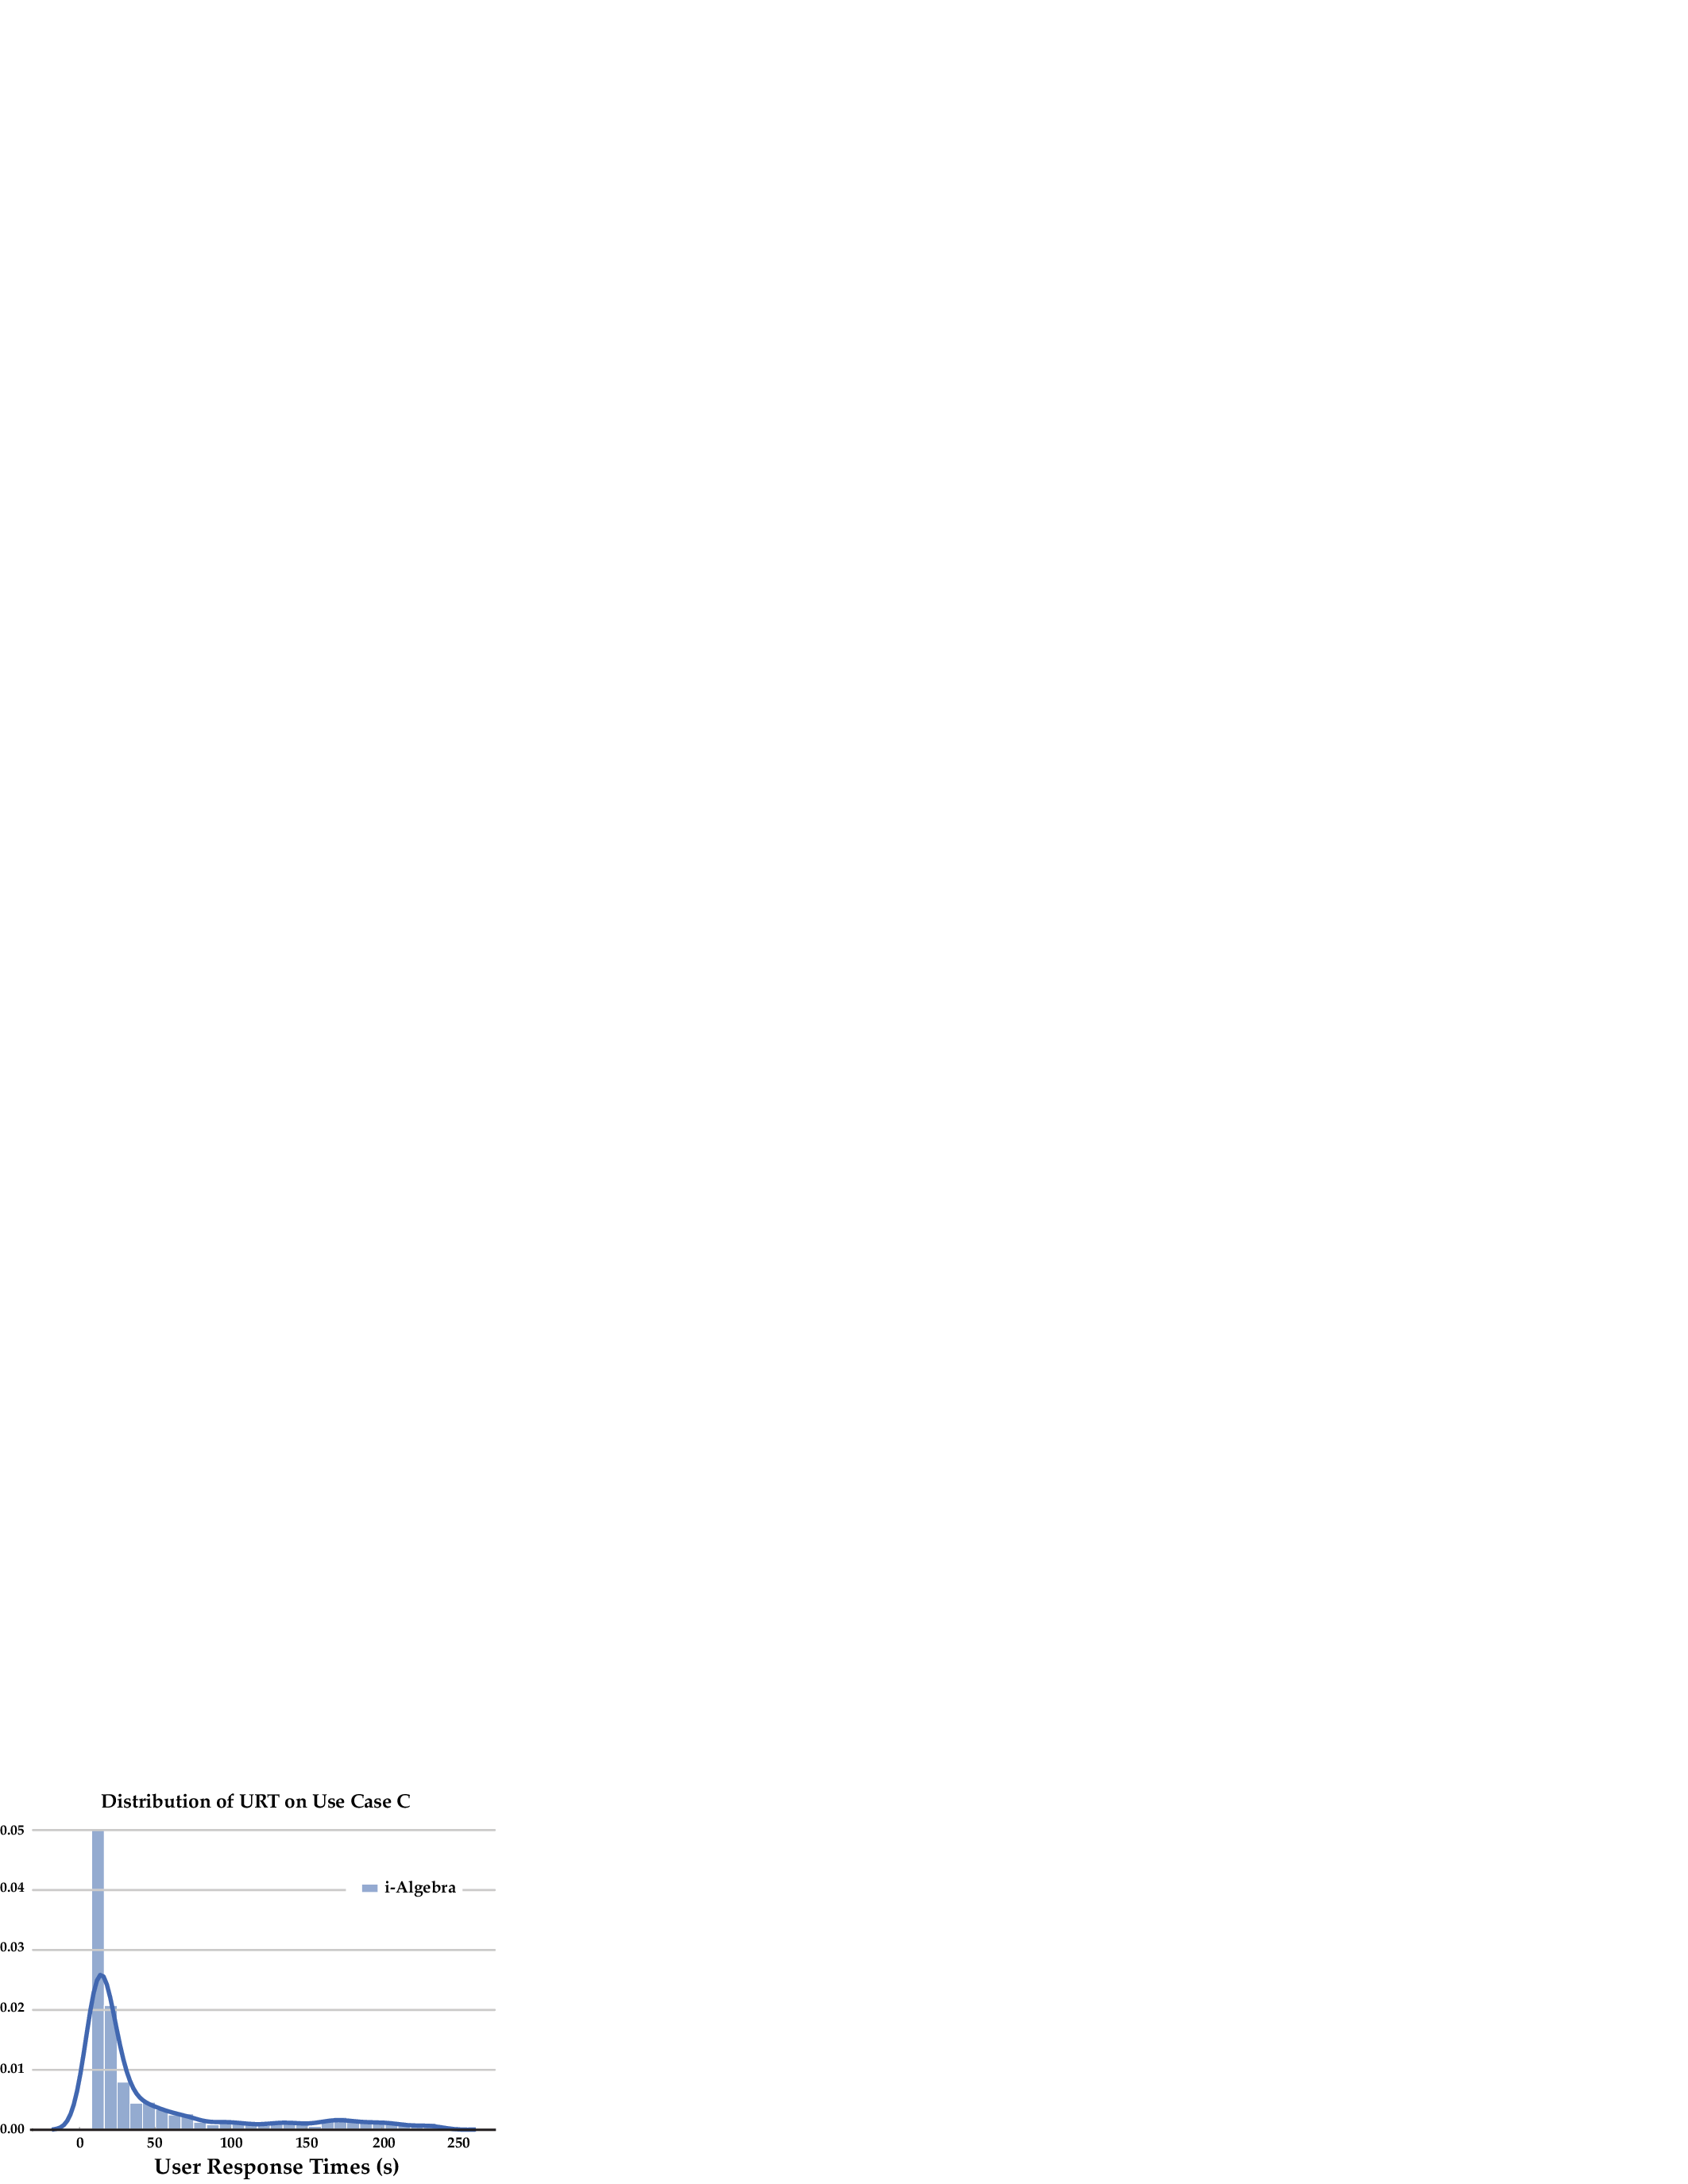, width=55mm}
% 	\caption{Distribution of URT in Case C. \label{fig:usecasec}}
% \end{figure*}
